# Supplementary material for: To Adapt or to Annotate: Challenges and Interventions for Domain Adaptation in Open-Domain Question Answering
Source: arXiv:2212.10381 source file (2022-12-20)
Supplement: Supplementary file 1 [file 7-appendix.tex]

\begin{table}[!htb]
\centering
    \small
    \begin{tabular}{lccccl}
    \toprule
      Dataset & \multicolumn{2}{c}{Retriever}  & \multicolumn{2}{c}{Reader} & {Shift} \\ 
      \cmidrule{2-3} \cmidrule{4-5} 
       & $d_u^t$ & $d_g^t$ & $d_u^t$ & $d_u^r - d_u^t$ \\
     \midrule
      BioASQ & 0.6477 & 0.3450 & 0.1160 & 0.1765 & Label \\ 
      CliCR & 0.0602 & 0.9448 & 0.0573 & 0.2352 & Full\\
      Quasar-S & 0.1658 & 0.8355 & 0.2158 &  0.0767 & Covar. \\ 
      Quasar-T & 0.5978 & 0.3962 & 0.1231 & 0.1694 & Label\\ 
      NewsQA  & 0.3992  &  0.5959 &  0.1125 & 0.1800 & Full\\ 
      SearchQA & 0.80350 & 0.1870 & 0.2988 & -0.0063 & No\\ 
    \bottomrule
    \end{tabular}
    \caption{Wasserstein distance computed over 100 examples with $d_u^r$=0.2925}
    \label{tab:ret_wd}
\end{table}
